# Supplementary material for: Neural Language Generation: Formulation, Methods, and Evaluation
Source: arXiv:2007.15780 source file (2020-07-31)
Supplement: Supplementary file 1 [file appendix.tex]

\appendix

%\clearpage
\section{Appendix A}
\label{AppendixA}

\begin{table*}[!htbp]
\caption{Overview of automatic evaluation metrics.}
\centering
\small
\scalebox{0.8}{
\begin{tabular}{ l| l| l | l}
\hline
\hline
\textbf{Type} & \textbf{Evaluation Metric} & \textbf{ Description} & \textbf{Reference}\\
\hline
\hline
\textit{n-gram based metrics} & BLEU  & & \cite{papineni2002bleu} \\
\hline
& SentBLEU  & & \cite{lin2004orange}, \cite{koehn2007moses} \\
\hline
& SacreBLEU & & \cite{post2018call} \\
\hline
& $\Delta$ BLEU  & & \cite{galley2015deltableu} \\
\hline
& ROUGE & & \cite{lin2004looking} \\
\hline
& ROUGE-$n$ & & \cite{lin2004looking} \\
\hline
& ROUGE-$L$ & & \\
\hline
& METEOR & & \cite{banerjee2005meteor} \\
\hline
& METEOR 1.5 & & \cite{denkowski2014meteor} \\
\hline
& METEOR++ 2.0 & & \cite{guo2019meteor} \\
\hline
& NIST & & \cite{doddington2002automatic} \\
\hline
& CIDEr & tf-idf weighted n-grams for similarity estimation & \cite{vedantam2015cider} \\
\hline
& SPICE & synonym matching over scene graphs &  \\
\hline
& LEIC & & \cite{cui2018learning} \\
\hline
& CHRF & & \cite{popovic2015chrf} \\
\hline
& CHRF ++ & & \cite{popovic2017chrf} \\
\hline
\textit{Distance based metrics} & Edit distance / Word error rate & & \cite{levenshtein1966binary} \\
\hline
& PER & & \cite{tillmann1997accelerated} \\
\hline
& CDER & & \cite{leusch2006cder} \\
\hline
& TER & & \cite{snover2006study} \\
\hline
& ITER & & \cite{panja2018iter} \\
\hline
& CharacTER & & \cite{wang2016character} \\
\hline
& EED & & \cite{stanchev2019eed} \\
\hline
\textit{Pre-trained metrics} & BERTscore & & \cite{zhang2019bertscore} \\
\hline
\textit{Fully learnt metrics} & BEER & & \cite{stanojevic2014beer} \\
\hline
\hline
\end{tabular}}
\label{table_compatibility}
\end{table*}
